# Supplementary material for: TadGAN: Time Series Anomaly Detection Using Generative Adversarial Networks
Source: arXiv:2009.07769 source file (2020-11-14)
Supplement: Supplementary file 1 [file appendix.tex]

\section{Appendix}
    See appendix.
 % Tighter
 \begin{table*}[!b]
%  \vspace{-1cm}
  \caption{Precision, Recall and F1-Scores of baseline models}
 \begin{tabulary}{\textwidth}{LLLLLLLLLLLLL}
 \toprule
  & & \multicolumn{2}{c}{NASA} & \multicolumn{4}{c}{Yahoo S5} & \multicolumn{5}{c}{NAB}  \\
   \cmidrule(r){3-4}\cmidrule(r){5-8}\cmidrule(r){9-13}
 \textbf{Variation} & & MSL & SMAP & A1 & A2 & A3 & A4 & Art & AdEx & AWS & Traf & Tweets\\
 \toprule
 & P    & 0.318 & 0.484 
        & 0.552 & 0.576 & 0.729 & 0.569 
        & 0.313 & 0.438 & 0.5 & 0.375 & 0.625 \\
 HTM    & R & 0.657 & 0.583 
        & 0.629 & 0.78 & 0.209 & 0.192
        & 0.833 & 0.636 & 0.667 & 0.643 & 0.455 \\
 & F1   & 0.557 & 0.412 
        & 0.588 & 0.662 & 0.325 & 0.287 
        & 0.455 & 0.519 & 0.571 & 0.474 & 0.526\\
 \hline
  & P   & 0.359 & 0.649
        & 0.689 & 0.975 & 0.987 & 0.896 
        & 0.3 & 0.467 & 0.474 & 0.481 & 0.514\\
 LSTM   & R & 0.639 & 0.758
        & 0.809 & 0.985 & 0.634 & 0.504 
        & 0.5 & 0.636 & 0.6 & 0.929 & 0.576\\
 & F1   & 0.46 & 0.699
        & 0.744 & 0.98 & 0.772 & 0.645 
        & 0.375 & 0.538 & 0.474 & 0.634 & 0.543\\
 \hline
 & P    & 0.356 & 0.368 
        & 0.648 & 0.747 & 0.997 & 0.938 
        & 0.273 & 0.538 & 0.4 & 0.462 & 0.559\\
 Arima  & R & 0.8 & 0.488 
        & 0.826 & 0.95 & 0.689 & 0.562
        & 0.5 & 0.636 & 0.733 & 0.75 & 0.576\\
 & F1   & 0.492 & 0.42 
        & 0.726 & 0.836 & 0.815 & 0.703 
        & 0.353 & 0.583 & 0.518 & 0.571 & 0.567\\
 \hline
 \multirow{3}{*}{\parbox{1.4cm}{Dense AE}} 
 & P    & 0.514 & 0.792 
        & 0.853 & 0.921 & 0.937 & 0.433 
        & 0.667 & 0.5 & 0.8 & 0.4 & 0.5\\
 & R    & 0.326 & 0.626 
        & 0.433 & 0.175 & 0.038 & 0.05
        & 0.333 & 0.182 & 0.533 & 0.286 & 0.03\\
 & F1   & 0.507 & 0.7
        & 0.472 & 0.294 & 0.074 & 0.09 
        & 0.444 & 0.267 & 0.64 & 0.333 & 0.057\\
 \hline
 \multirow{3}{*}{\parbox{1.4cm}{LSTM AE}} 
 & P    & 0.514 & 0.657 
        & 0.656 & 0.848 & 0.9 & 0.599 
        & 0.6 & 0.6 & 0.84 & 0.533 & 0.615\\
 & R    & 0.5 & 0.687 
        & 0.567 & 0.895 & 0.144 & 0.095 
        & 0.5 & 0.545 & 0.7 & 0.571 & 0.485\\
 & F1   & 0.507 & 0.672 
        & 0.608 & 0.871 & 0.248 & 0.163 
        & 0.545 & 0.571 & 0.764 & 0.552 & 0.542\\
 \hline
  \multirow{3}{*}{\parbox{1.4cm}{MAD-GAN}} 
 & P    & 0.167 & 0.222
        & 0.253 & 0.296 & 0.502 & 0.321 
        & 0.193 & 0.174 & 0.16 & 0.259 & 0.309\\
 & R    & 0.083 & 0.09 
        & 0.68 & 0.848 & 0.709 & 0.834 
        & 1 & 1 & 0.9 & 1 & 0.787 \\
 & F1   & 0.111 & 0.128 
        & 0.369 & 0.439 & 0.588 & 0.463 
        & 0.324 & 0.297 & 0.273 & 0.412 & 0.444\\
 \hline
 \multirow{3}{*}{\parbox{1.4cm}{MS Azure}} 
 & P    & 0.167 & 0.129 
        & 0.328 & 0.64 & 0.64 & 0.41 
        & 0.114 & 0.21 & 0.189 & 0.313 & 0.159 \\
 & R    & 0.314 & 0.1 
        & 0.638 & 0.648 & 0.169 & 0.194
        & 0.194 & 0.058 & 0.176 & 0.146 & 0.106 \\
 & F1   & 0.218 & 0.118 
        & 0.352 & 0.612 & 0.257 & 0.204
        & 0.125 & 0.066 & 0.173 & 0.166 & 0.118 \\
 \hline
 \multirow{3}{*}{\parbox{1.4cm}{DeepAR}} 
 & P    & 0.617 & 0.436 
        & 0.664 & 0.913 & 0.926 & 0.9 
        & 0.6   & 0.533 & 0.308 & 0.563 & 0.615 \\
 & R    & 0.552 & 0.472
        & 0.444 & 0.945 & 0.313 & 0.303 
        & 0.5   & 0.727 & 0.533 & 0.643 & 0.485 \\
 & F1   & 0.583 & 0.453
        & 0.532 & 0.929 & 0.467 & 0.454
        & 0.545 & 0.615 & 0.39  & 0.6 & 0.542 \\
 \toprule
 \end{tabulary}
 \vspace{-0.5cm}
 \label{tab:Baselines_appendix}
 \end{table*}
